# Supplementary material for: MAMBA4D: Efficient Long-Sequence Point Cloud Video Understanding with Disentangled Spatial-Temporal State Space Models
Source: arXiv:2405.14338 source file (2025-02-27)
Supplement: Supplementary file 1 [file X_suppl.tex]

\clearpage
\setcounter{page}{1}
\maketitlesupplementary

\section{Overview}
The supplementary materials are structured as follows:
\begin{itemize}
\item We give more detailed illustrations about the dataset for 4D tasks in Section \ref{sec:data};
\item More descriptions about the loss functions are provided in Section \ref{sec:loss}.
\item We analyze the error bar of the prediction accuracy in Section \ref{sec:exp} and display more visualization results in Section \ref{sec:visual}.
\end{itemize}

\section{Datasets}
\label{sec:data}
\textbf{MSR-Action3D.} The MSR-Action3D dataset \cite{li2010action} is composed of 567 Kinect depth videos, including 20 action categories and 23K frames in total. We partition the train/test split following \cite{fan2021pstnet,fan2021point}, and sample 2048 points for each frame. Only point coordinates are available without point colors. Point cloud videos are partitioned into multiple equal-size clips. Video-level labels are directly used as clip-level labels when training. For testing, the mean of clip-level predicted probabilities is viewed as the video ones.

\vspace{3pt}
\noindent\textbf{HOI4D.} The HOI4D dataset \cite{liu2022hoi4d} contains 2,971 training videos and 892 test videos for action segmentation. Each video sequence has 150 frames with each frame containing 2048 points. The dataset contains a total of 579K frames. All frames are annotated with 19 fine-grained action classes in the interactive scene.

\vspace{3pt}
\noindent\textbf{Synthia 4D.} The Synthia 4D \cite{choy20194d} dataset is generated from the Synthia dataset \cite{ros2016synthia}, including 6 driving scene videos. Each video consists of 4 stereo RGB-D images captured from the top of the car. 3D point cloud videos are obtained from RGB and depth images. We follow \cite{fan2021point} to split the training (19888 frames)/  validation (815 frames)/ test (1886 frames) sets. The evaluation metric is the mean Intersection over Union (mIoU).

\begin{figure}[t]
\centering
\includegraphics[width=0.8\linewidth]{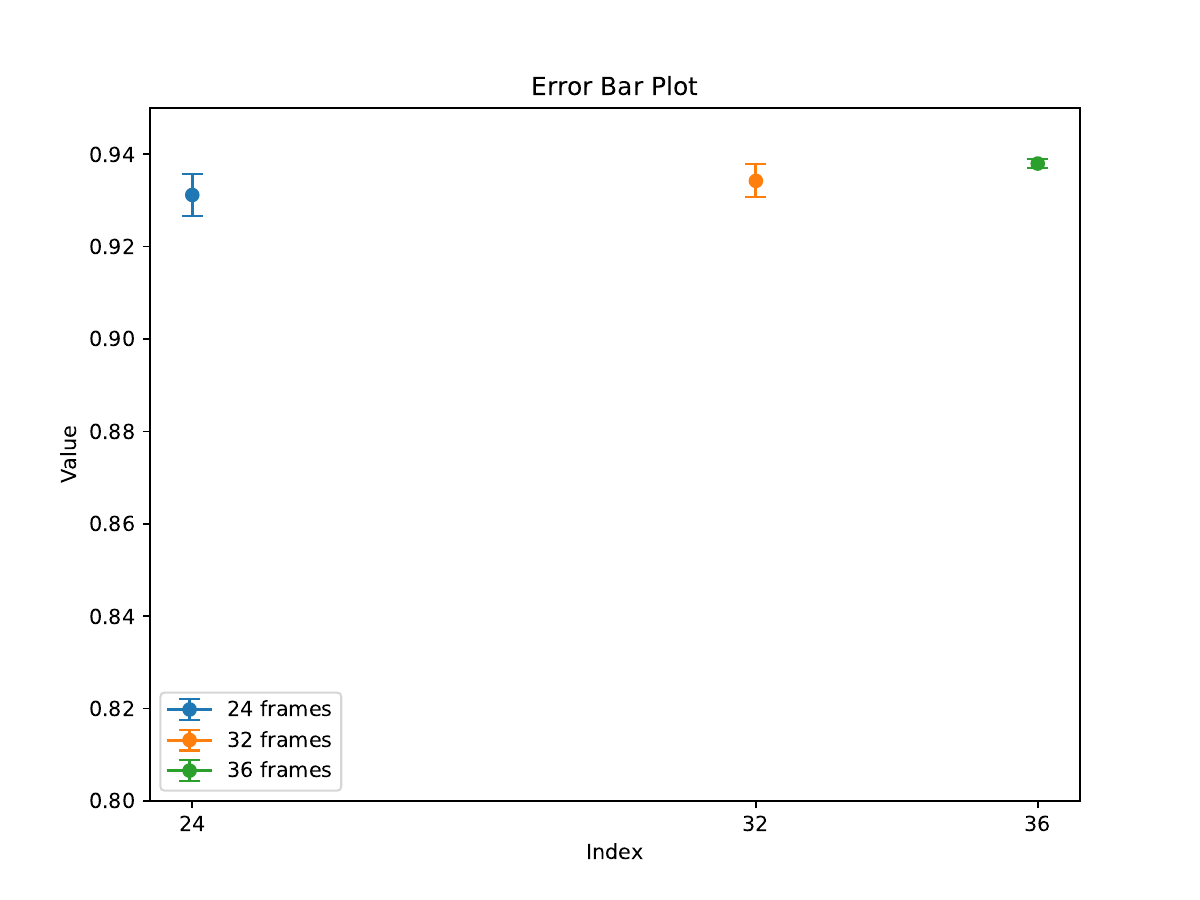}
%\vspace{-7mm}
\caption{\textbf{Error bars of our estimated action recognition accuracy for 24, 32, and 36 frames as inputs.} We can see a stable performance with a small fluctuation around the mean accuracy.}
\label{fig:visual1}
\end{figure}

\section{Loss Functions}
\label{sec:loss}
\textbf{3D Action Recognition.} In this task, the model is trained to classify a sequence of video frames into predefined action categories. The primary loss function employed is the Cross-Entropy Loss, which is defined as follows:
\begin{equation}
\mathcal{L} = - \Sigma_{i=1}^{N} y_i \log(p_i),
\end{equation}
where \(N\) is the total number of videos, \(y_i\) is the true label for the \(i\)-th class and \(p_i\) is the predicted probability for the \(i\)-th class. The loss function supervises the model by providing a scalar value that quantifies the discrepancy between the predicted action probabilities and the true action labels. During the training process, the model parameters are optimized to minimize this loss value. 

\textbf{4D Action Segmentation.} In the task of 4D action segmentation, the goal is to classify frames in a point cloud sequence into action categories. The primary loss function employed is the Cross-Entropy Loss, defined as:
\begin{equation}
\mathcal{L} = - \Sigma_{i=1}^{N} y_i \log(p_i),
\end{equation}
where \(N\) represents the total number of frames in the point cloud sequence, \(y_i\) is the true action label for the \(i\)-th frame, and \(p_i\) is the predicted probability for the corresponding action class. This loss function measures the prediction error between the predicted and ground truth action labels across the point cloud sequence frames.

\textbf{4D Semantic Segmentation.} In the task of 4D semantic segmentation, the goal is to classify each point in a sequence of point clouds into semantic categories. The primary loss function employed in this task is the weighted Cross-Entropy Loss, which is defined as follows:
\begin{equation}
\mathcal{L} = - \Sigma_{i=1}^{N} w_i y_i \log(p_i),
\end{equation}
where \(N\) is represents the total number of points in the point cloud, \(w_i\) is the weight for the \(i\)-th class to handle class imbalance, \(y_i\) is the true label for the \(i\)-th point, and the \(p_i\) is the predicted probability for the \(i\)-th class. The loss function supervises the 4D semantic segmentation task by providing a measure of the prediction error between the predicted semantic labels and the true labels for each point in the point cloud.

\begin{figure*}[t]
\centering
\includegraphics[width=1.0\linewidth]{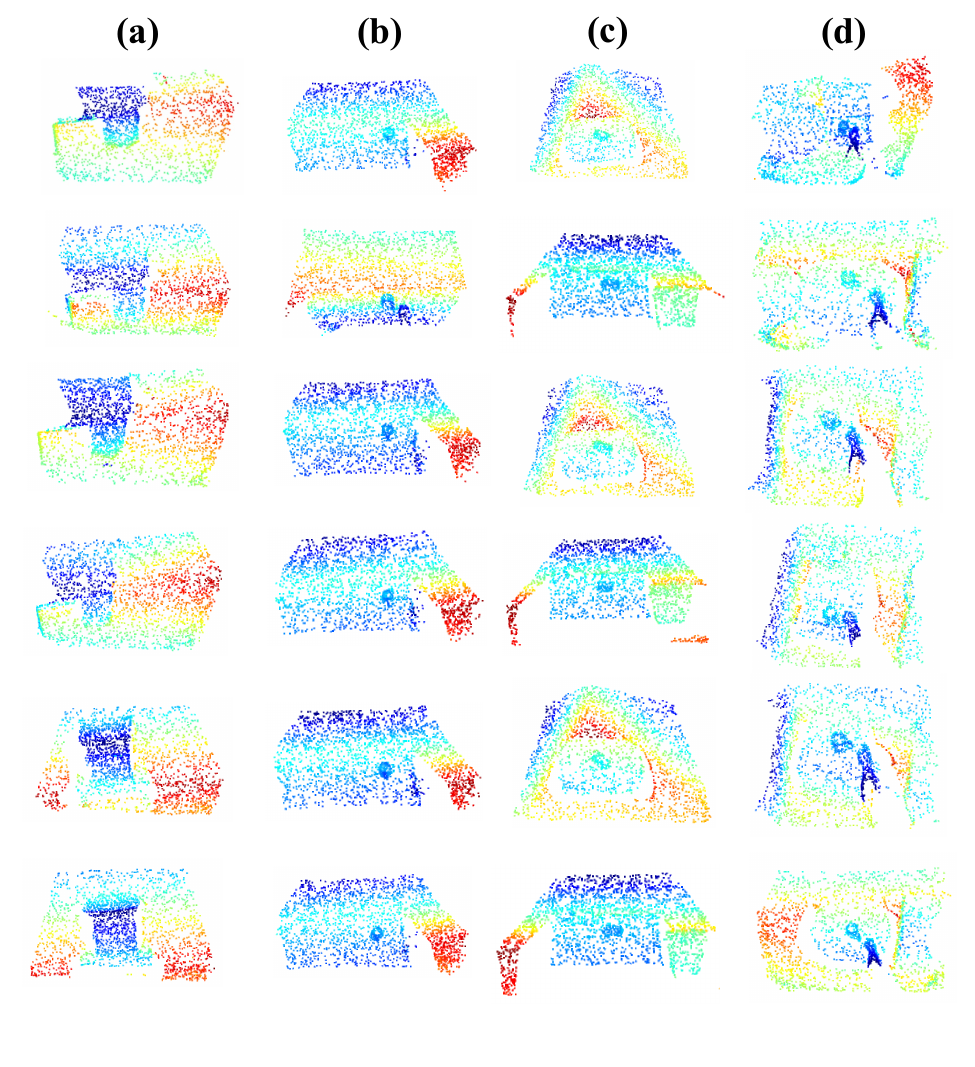}
%\vspace{-7mm}
\caption{\textbf{More visualization samples of the 4D action segmentation.}}
\label{fig:visual2}
\end{figure*}

\begin{figure*}[t]
\centering
\includegraphics[width=0.8\linewidth]{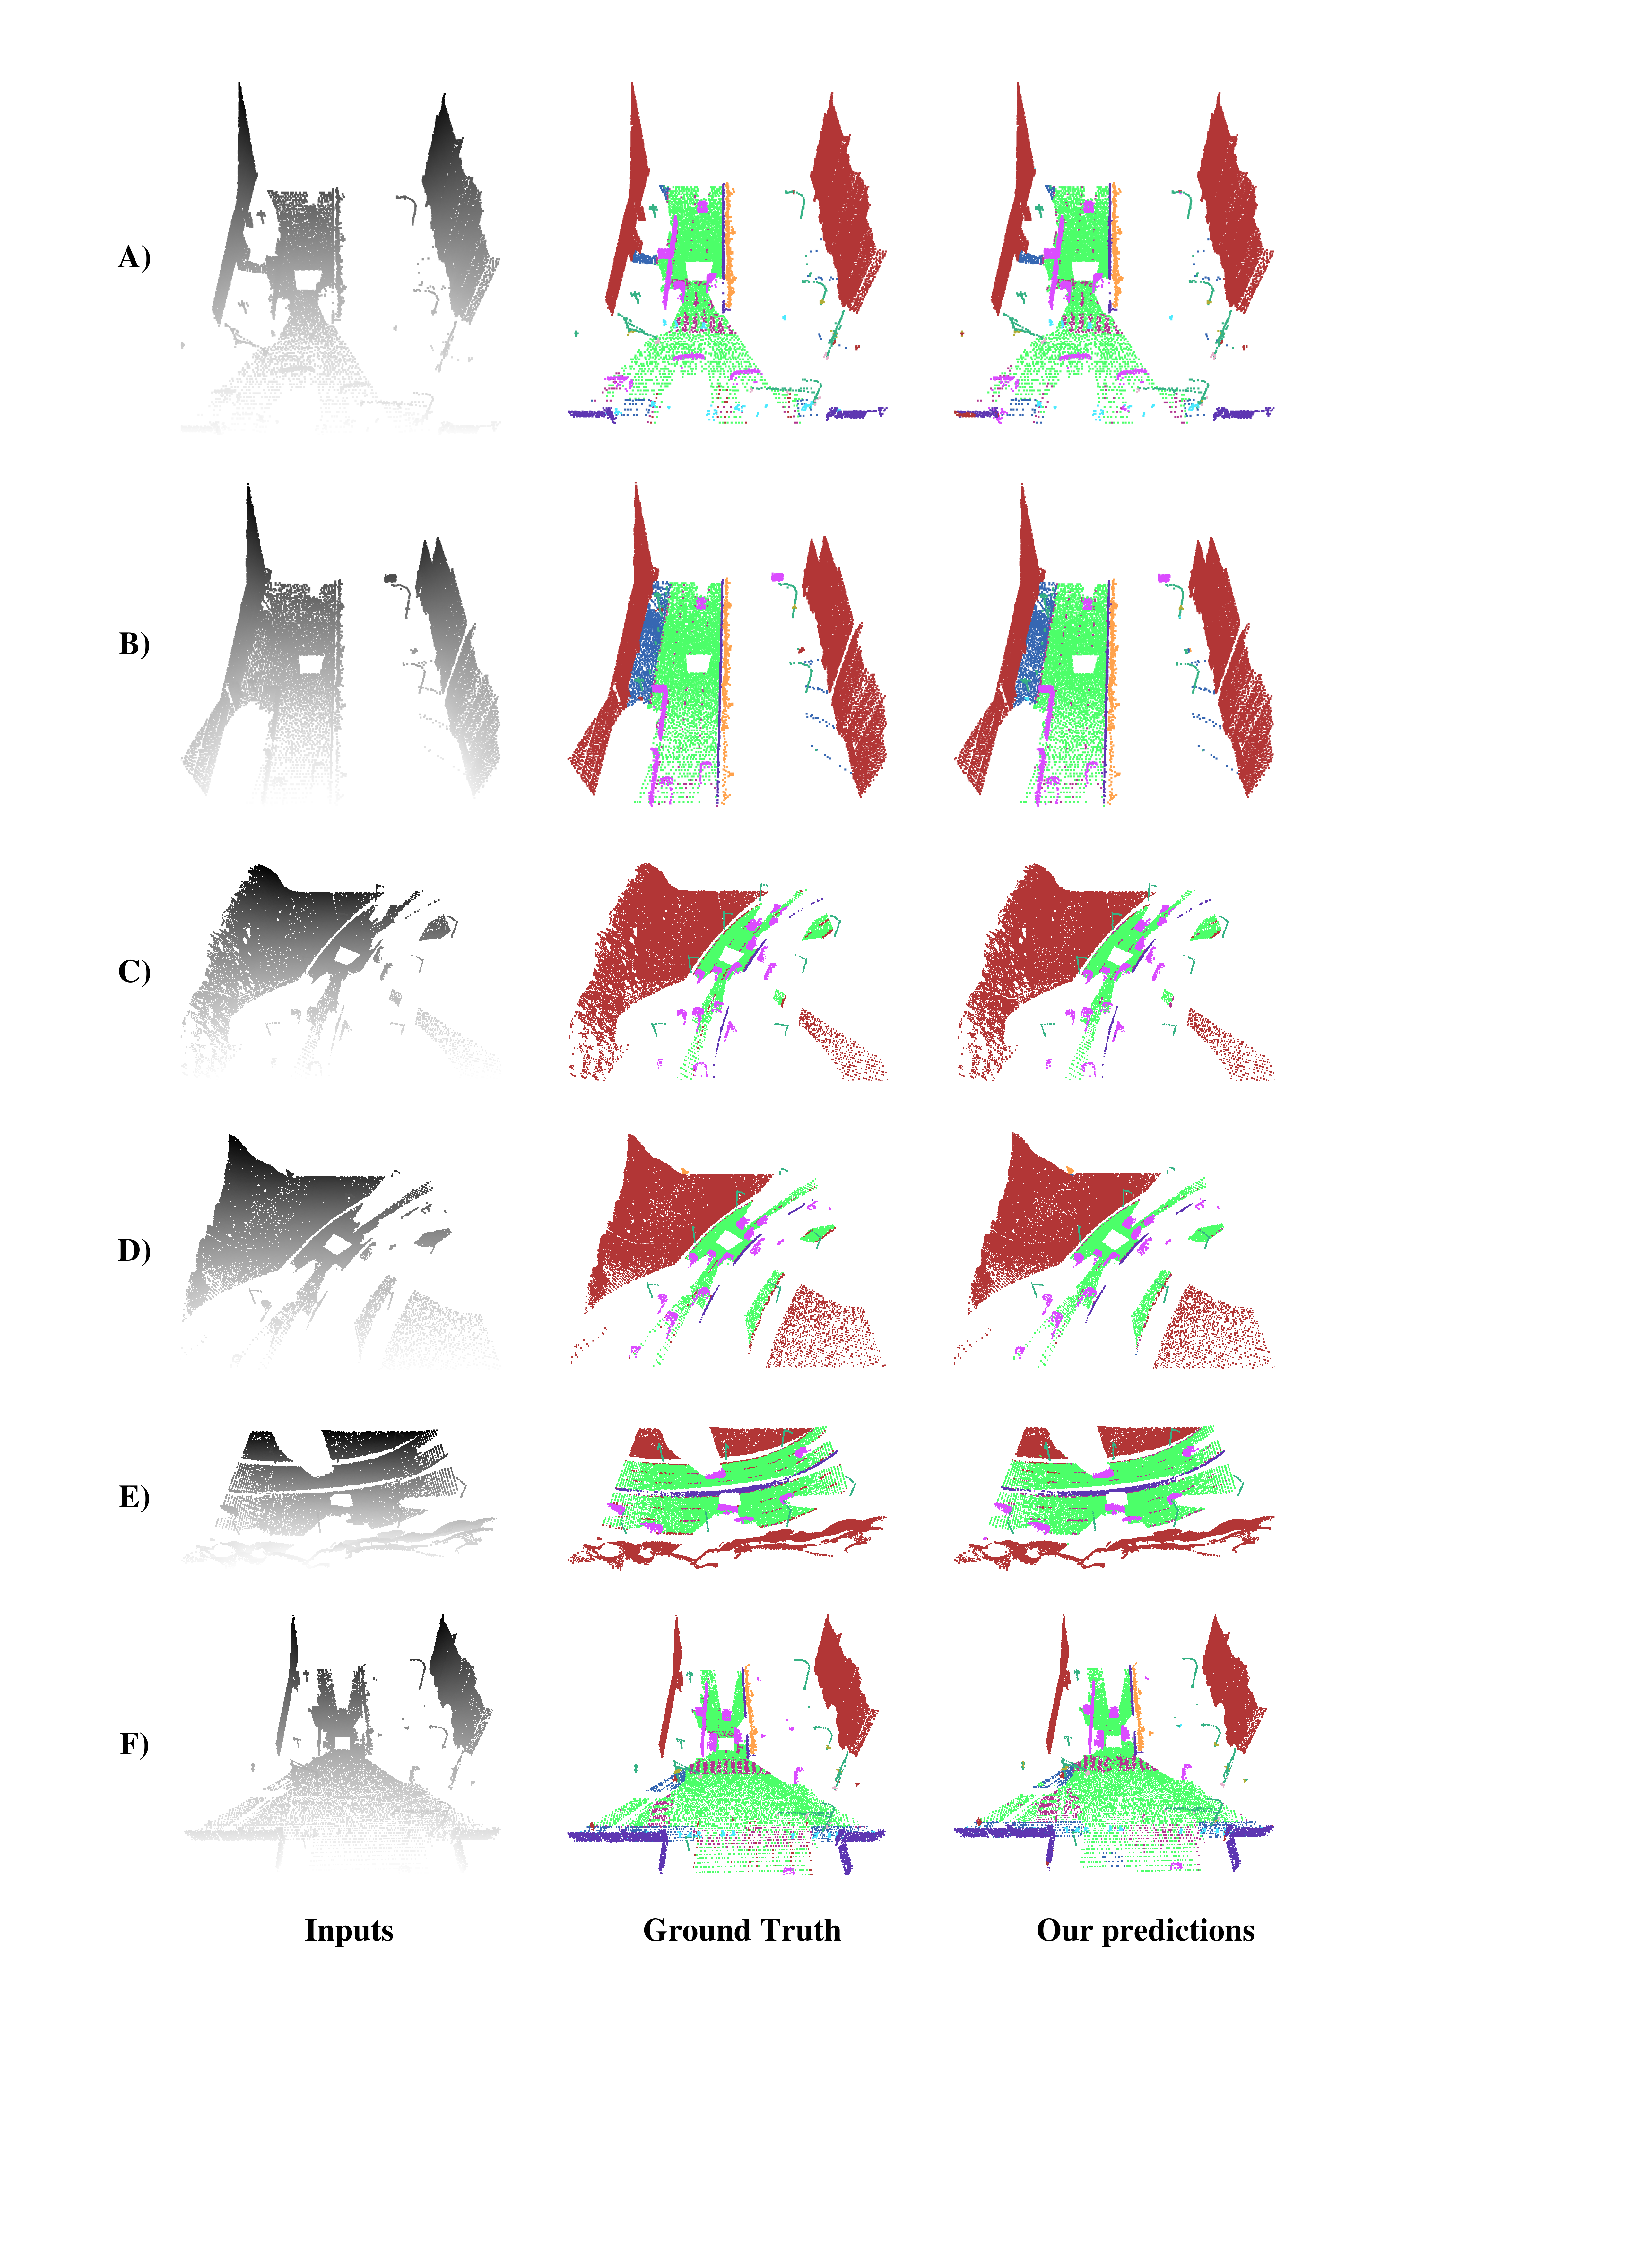}
%\vspace{-7mm}
\caption{\textbf{More visualization samples of the 4D semantic segmentation.}}
\label{fig:visual3}
\end{figure*}

\section{Error Bar Analysis}
\label{sec:exp}
We plot the error bar about the action recognition accuracy for 24, 32, and 36 frames as inputs in Fig .\ref{fig:visual1}. From the figure, we can see a stable performance with a small fluctuation around the mean accuracy.

\section{Visualization}
\label{sec:visual}
We show more visualization results in  Fig. \ref{fig:visual2} and Fig. \ref{fig:visual3} respectively for the 4D action segmentation and semantic segmentation. In Fig. \ref{fig:visual3}, all the predicted segmentation labels are highly overlapped with the Ground Truth, which shows the perfect accuracy of our method.
