# Supplementary material for: MAMBA4D: Efficient Long-Sequence Point Cloud Video Understanding with Disentangled Spatial-Temporal State Space Models
Source: arXiv:2405.14338 source file (2025-02-27)
Supplement: Supplementary file 2 [file supp.tex]

\textbf{HOI4D} The HOI4D dataset \cite{liu2022hoi4d} contains 2,971 training videos and 892 test videos for action segmentation. Each video sequence has 150 frames with each frame containing 2048 points. The dataset contains a total of 579K frames. All frames are annotated with 19 fine-grained action classes in the interactive scene.

\textbf{4D Action Segmentation.} In the task of 4D action segmentation, the goal is to classify frames in a point cloud sequence into action categories. The primary loss function employed is the Cross-Entropy Loss, defined as:
\begin{equation}
\mathcal{L} = - \Sigma_{i=1}^{N} y_i \log(p_i),
\end{equation}
where \(N\) represents the total number of frames in the point cloud sequence, \(y_i\) is the true action label for the \(i\)-th frame, and \(p_i\) is the predicted probability for the corresponding action class. This loss function measures the prediction error between the predicted and true action labels across the point cloud sequence frames.
